# Supplementary material for: Process Bigraphs and the Architecture of Compositional Systems Biology
Source: arXiv:2512.23754 source file (2026-08-14)
Supplement: Supplementary file 1 [file supp.tex]

\documentclass[letterpaper,11pt]{article}

% Basic packages
\usepackage[margin=1in]{geometry}
\usepackage{setspace}
\usepackage{graphicx}
\usepackage{amsmath, amssymb}
\usepackage{hyperref}
\usepackage{xcolor}
\usepackage{listings}
\usepackage{float}
\usepackage{caption}

\usepackage{biblatex}
\usepackage{authblk}
\usepackage{enumitem}
\usepackage{xspace}
\usepackage{varwidth} % optional, but helps keep boxes narrow
% \usepackage{longtable}

% Code listings look similar to Vivarium 2021 supplement
\lstset{
    basicstyle=\ttfamily\small,
    breaklines=true,
    frame=single
}

% --- Pretty type block environment ---
\usepackage{varwidth} % optional, but helps keep width tight
\usepackage{mdframed}

% ------------------------------------------------------------
% TYPE CARD HEADER
% #1 = type name (e.g. conc_counts)
% #2 = human-readable title
% #3 = store category label (e.g. "fields", "particles", "global_time", etc.)
% ------------------------------------------------------------
\newenvironment{sfxtypecard}[3]%
{%
  \begin{mdframed}[
      backgroundcolor=gray!4,
      linecolor=gray!50,
      roundcorner=3pt,
      innertopmargin=0.8em,
      innerbottommargin=0.8em,
      innerleftmargin=1em,
      innerrightmargin=1em
    ]
    \noindent\ignorespaces
    {\bfseries #2}%
    \hfill{\small\textsf{#3}}%
    \par\vspace{0.4em}%
}%
{%
  \end{mdframed}%
  \vspace{0.8em}%
}

% ------------------------------------------------------------
% FIELDS TABLE 
% ------------------------------------------------------------
\newenvironment{sfxtypefields}[1]%
{%
  \par\vspace{0.2em}%
  \vspace{0.2em}%
  \begin{center}%
    \renewcommand{\arraystretch}{1.2}%
    \begin{tabular}{p{0.35\textwidth} p{0.5\textwidth}}%
      \hline
      \multicolumn{2}{l}{\textbf{\texttt{type #1}}} \\
      \hline
      \textbf{Field} & \textbf{Type} \\
      \hline
}%
{%
      \hline
    \end{tabular}%
  \end{center}%
  \vspace{0.4em}%
}

\newcommand{\sfxfieldrow}[2]{%
  #1 & #2\\%
}

% ------------------------------------------------------------
% PROCESS CARDS
% #1 = internal name (particle_exchange)
% #2 = human-readable title
% #3 = kind: process | step
% #4 = category label: metabolic | field | particle movement | bridge | graph rewrite | ...
% ------------------------------------------------------------
\newenvironment{sfxprocesscard}[4]{%
  \begin{mdframed}[linewidth=0.4pt,roundcorner=2pt,backgroundcolor=gray!5]%
    \noindent\ignorespaces
    \textbf{#2}%
    \hfill{\small\textsf{#4}}%
    \par\vspace{0.5\baselineskip}%
}{%
  \end{mdframed}%
  \vspace{0.8em}%
}

% ------------------------------------------------------------
% PROCESS INTERFACE TABLE
% Usage:
% \begin{sfxprocessinterface}{monod_kinetics}{process}
%   \sfxprocport{biomass}{input}{concentration}
%   ...
% \end{sfxprocessinterface}
%
% This puts "process monod_kinetics" in the header row, mirroring type tables.
% ------------------------------------------------------------
\newenvironment{sfxprocessinterface}[2]{%
  \par\vspace{0.4em}%
  \noindent\textbf{Interface}\par
  \vspace{0.2em}%
  \begin{center}%
    \renewcommand{\arraystretch}{1.2}%
    \begin{tabular}{p{0.27\textwidth} p{0.22\textwidth} p{0.41\textwidth}}%
      \hline
      \multicolumn{3}{l}{\textbf{\texttt{#2 #1}}} \\
      \hline
      \textbf{Name} & \textbf{Direction} & \textbf{Type} \\
      \hline
}{%
      \hline
    \end{tabular}%
  \end{center}%
  \vspace{0.4em}%
}

\newcommand{\sfxprocport}[3]{%
  #1 & #2 & #3\\%
}

% ------------------------------------------------------------
% PROCESS PARAMETER TABLE
% ------------------------------------------------------------
\newenvironment{sfxprocessparams}{%
  \par\vspace{0.1em}%
  \noindent\textbf{Parameters}\par
  \vspace{0.2em}%
  \begin{center}%
    \renewcommand{\arraystretch}{1.2}%
    % 0.24 + 0.19 + 0.15 + 0.30 = 0.88 < available width inside mdframed
    \begin{tabular}{p{0.24\textwidth} p{0.19\textwidth} p{0.15\textwidth} p{0.30\textwidth}}%
      \hline
      \textbf{Parameter} & \textbf{Type} & \textbf{Default} & \textbf{Role} \\
      \hline
}{%
      \hline
    \end{tabular}%
  \end{center}%
  \vspace{0.4em}%
}

\newcommand{\sfxprocparam}[4]{%
  #1 & #2 & #3 & #4\\%
}

% ============================================================
% COMPOSITE CARD
% ============================================================
% One small card, labeled only with the composite name in the top right
% #1 = composite name (particle_comets)
\newenvironment{sfxcompositecard}[1]{%
  \begin{mdframed}[linewidth=0.4pt,
                   roundcorner=2pt,
                   backgroundcolor=gray!3,
                   skipabove=0.8em,
                   skipbelow=0.8em]%
    \noindent\hfill{\small\texttt{composite #1}}%
    \par\vspace{0.5\baselineskip}%
}{%
  \end{mdframed}%
}

% ============================================================
% STORES TABLE
% ============================================================
% Usage:
% \begin{sfxcompositestores}
%   \sfxstore{fields}{map[array[conc_counts_volume]]}
%   ...
% \end{sfxcompositestores}

% ============================================================
% PROCESSES SECTION + PROCESS HEADER
% ============================================================
% #1 = instance label (e.g. monod_kinetics[0,0])
% #2 = kind+name (e.g. process monod_kinetics)
% #3 = category label (e.g. metabolic, field, particle movement)
\newenvironment{sfxcompositeprocess}[3]{%
  \vspace{0.4em}%
  \noindent\textbf{#1}\hfill{\small\textsf{#3}}\\%
  {\small\texttt{#2}}%
  \par\vspace{0.3em}%
}{%
  \vspace{0.4em}%
}

% ============================================================
% WIRES TABLE
% ============================================================
% Usage:
% \begin{sfxcompositewires}
%   \sfxwire{fields}{input}{fields}
%   ...
% \end{sfxcompositewires}
\newenvironment{sfxcompositewires}{%
  \noindent\textbf{Wiring}\par\vspace{0.2em}%
  \renewcommand{\arraystretch}{1.15}%
  \begin{center}%
    \begin{tabular}{p{0.26\textwidth} p{0.22\textwidth} p{0.40\textwidth}}%
      \hline
      \textbf{Port} & \textbf{Direction} & \textbf{Store path} \\
      \hline
}{%
      \hline
    \end{tabular}%
  \end{center}%
  \vspace{0.3em}%
}

\newcommand{\sfxwire}[3]{%
  \texttt{#1} & #2 & \texttt{#3}\\%
}

% ============================================================
% PROCESS PROPERTIES TABLE
% ============================================================
% Usage:
% \begin{sfxcompositeprops}
%   \sfxprop{interval}{1.0}
%   \sfxprop{address}{local.DiffusionAdvection}
% \end{sfxcompositeprops}
\newenvironment{sfxcompositeprops}{%
  \noindent\textbf{Properties}\par\vspace{0.2em}%
  \renewcommand{\arraystretch}{1.15}%
  \begin{center}%
    \begin{tabular}{p{0.32\textwidth} p{0.56\textwidth}}%
      \hline
      \textbf{Property} & \textbf{Value} \\
      \hline
}{%
      \hline
    \end{tabular}%
  \end{center}%
  \vspace{0.3em}%
}

\newcommand{\sfxprop}[2]{%
  #1 & \texttt{#2}\\%
}

% ============================================================
% CONFIG TABLE 
% ============================================================
% Usage:
% \begin{sfxconfigtable}
%   \sfxconfigrow{n_bins}{[2, 2]}
%   ...
% \end{sfxconfigtable}
\newenvironment{sfxconfigtable}{%
  \noindent\textbf{Config}\par\vspace{0.2em}%
  \renewcommand{\arraystretch}{1.15}%
  \begin{center}%
    \begin{tabular}{p{0.46\textwidth} p{0.42\textwidth}}%
      \hline
      \textbf{Key} & \textbf{Value} \\
      \hline
}{%
      \hline
    \end{tabular}%
  \end{center}%
  \vspace{0.4em}%
}

\newcommand{\sfxconfigrow}[2]{%
  \texttt{#1} & \texttt{#2}\\%
}

% ============================================================
% Title Page
% ============================================================

\title{
    Supplement for\\[6pt]
    \textbf{Process Bigraphs and the Architecture of\\
    Compositional Systems Biology}
}

\author{
    Eran Agmon\,
    \href{https://orcid.org/0000-0003-1279-2474}{\includegraphics[scale=0.04]{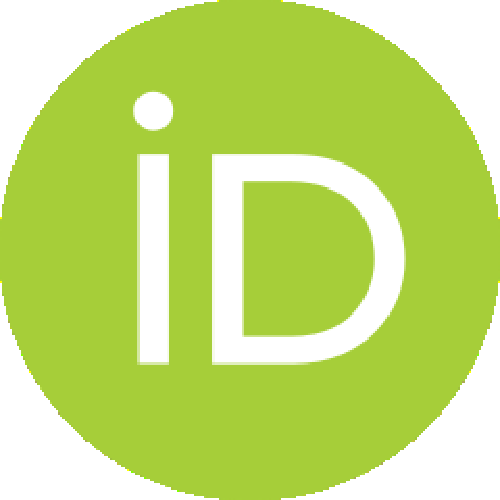}}
    \thanks{Correspondence: agmon@uchc.edu}
    \qquad
    Ryan K. Spangler\,
    \href{https://orcid.org/0000-0002-6080-3142}{\includegraphics[scale=0.04]{orcidicon.eps}}
}

\affil{
    Center for Cell Analysis and Modeling,\\
    University of Connecticut Health,\\
    Farmington, Connecticut, USA
}

\date{\today}

\begin{document}

\maketitle

\tableofcontents

% ============================================================
% S0. INTRODUCTION
% ============================================================

\section{Introduction}
\label{sec:supp-intro}

This supplementary materials document for ``Process Bigraphs and the Architecture of Compositional Systems Biology'' provides the technical underpinnings of the Process--Bigraph framework introduced in the main text.
Our goals are to
(i) make the semantics of Process--Bigraphs precise,
(ii) connect these abstract definitions to concrete Python classes in the Vivarium~2.0 software stack, and
(iii) illustrate the framework on a fully worked example (Spatio--Flux).

We proceed with the following sections:
\begin{itemize}[noitemsep,topsep=2pt,leftmargin=1.5em]
    \item Section~\ref{sec:software-suite} introduces the Vivarium~2.0 software suite, the core libraries used in this work, and the main runtime classes we refer to in the rest of the supplement.
    \item Section~\ref{sec:process-bigraphs} develops the formal, schema-based semantics of Process--Bigraphs in an implementation-agnostic way, but with direct correspondence to the classes and type registries provided by the software libraries.
    \item Section~\ref{sec:pb-spatioflux-instantiation} gives a detailed Spatio--Flux instantiation of these semantics, showing how field dynamics, stochastic/deterministic particle movement dynamics, and coupled particle--field metabolism are represented as Process--Bigraphs and executed by the Vivarium~2.0 stack.
\end{itemize}

% ============================================================
% S2. VIVARIUM 2.0 SOFTWARE SUITE
% ============================================================

\section{Vivarium~2.0 software suite}
\label{sec:software-suite}

The Vivarium~2.0 software suite provides the reference implementation of Process--Bigraphs used in this paper.
It consists of three core libraries and an application repository:

\begin{itemize}[noitemsep,topsep=2pt,leftmargin=1.5em]
    \item \textbf{\texttt{bigraph-schema}}: a foundational library that defines a compositional type system and hierarchical data structures using JSON-based schemas.
    It provides the \emph{type engine} (e.g.\ \texttt{Core}) and a global \texttt{type\_registry} that together implement:
    (i) schema compilation to path-addressed schema trees,
    (ii) validation of state trees, and
    (iii) type-specific update operators $\mathsf{apply}$ used in the delta semantics of Section~\ref{sec:process-bigraphs}.

    \item \textbf{\texttt{process-bigraph}}: the dynamic core of the framework.
    It defines:
    \begin{itemize}[noitemsep,topsep=0pt,leftmargin=1.5em]
        \item the \texttt{Process} and \texttt{Step} classes, which implement typed \emph{process nodes} with input/output ports, configuration, and an \texttt{address} used to look up their implementation;
        \item the \texttt{Composite} class, which encapsulates an entire process--bigraph as a single process with an explicit interface;
        \item the event-scheduling and orchestration logic that maintains a global time, an update schedule, and the repeated evaluation of process handlers.
    \end{itemize}

    \item \textbf{\texttt{bigraph-viz}}: a visualization library that parses the JSON representation of a process--bigraph and renders it as a graph.
\end{itemize}

\noindent
In addition to the core libraries, we use a domain-specific application repository:
\begin{itemize}[noitemsep,topsep=2pt,leftmargin=1.5em]
    \item \textbf{\texttt{spatio-flux}}: a complete multiscale example built on \texttt{process-bigraph} and \texttt{bigraph-schema} that defines a \texttt{Process} and \texttt{Composite} subclasses for: metabolic processes, field dynamics, particle dynamics, and coupled particle--field interactions.
    The repository includes an extended test suite that runs dozens of process--bigraph documents, some of which are referenced in Section~\ref{sec:pb-spatioflux-instantiation} as concrete instances of the abstract semantics.
\end{itemize}

\noindent
All source code, documentation, tutorials, and examples are available on the Vivarium Collective GitHub:
\begin{itemize}[noitemsep,topsep=2pt,leftmargin=1.5em]
    \item \texttt{process-bigraph}: \url{https://github.com/vivarium-collective/process-bigraph}
    \item \texttt{bigraph-schema}: \url{https://github.com/vivarium-collective/bigraph-schema}
    \item \texttt{bigraph-viz}: \url{https://github.com/vivarium-collective/bigraph-viz}
    \item \texttt{spatio-flux}: \url{https://github.com/vivarium-collective/spatio-flux}
\end{itemize}

% ============================================================
% S2. PROCESS–BIGRAPHS Semantics
% ============================================================

\section{Process--Bigraphs Semantics}
\label{sec:process-bigraphs}

This section develops the formal, schema-based semantics of Process--Bigraphs, expressed in a set-theoretic, function-based language.
We proceed from mathematical preliminaries to types, states, wiring, processes, composites, and orchestration.
Section~\ref{sec:pb-spatioflux-instantiation} then mirrors this general account with a Spatio--Flux-specific instantiation, so that readers can move back and forth between abstract definitions and concrete examples.

% ------------------------------------------------------------
% 2.1 Mathematical Preliminaries
% ------------------------------------------------------------

\subsection{Mathematical preliminaries}
\label{sec:pb-preliminaries}

A bigraph is organized as a hierarchical \emph{tree} (or, more generally, a forest) whose nodes are addressed by finite paths.
This representation matches naturally with JSON: objects correspond to nodes with children keyed by field names, arrays correspond to nodes with children keyed by integer indices, and following a sequence of keys or indices selects a unique location in the structure.

Let $\mathcal{M}$ be the set of \emph{marks} (atomic path components), and let
\[
    \mathcal{P} = \mathcal{M}^{\ast}
\]
be the set of finite paths, implemented as lists of marks (e.g.\ \texttt{["organism", "cell", "mass"]}).
% We write $p \cdot m$ for appending a mark $m$ to a path $p$, and use the standard prefix order $p \preceq q$ when $q$ begins with $p$.

Any JSON-like hierarchical structure induces a tree of such paths: objects and arrays correspond to internal nodes, and primitive values correspond to leaves.
In this supplement, both schemas and states are treated as partial maps from paths in $\mathcal{P}$ to types or values, respectively.

We can fix:
\begin{itemize}[noitemsep,topsep=2pt,leftmargin=1.5em]
    \item a set of types $\mathcal{T}$,
    \item a set of values $\mathcal{V}$,
    \item a subset of paths $\mathsf{StorePath} \subseteq \mathcal{P}$ that designate locations where concrete values may be stored.
\end{itemize}

% ------------------------------------------------------------
% 2.2 Serialized and Textual Representations
% ------------------------------------------------------------
\subsection{Serialized and human-readable forms}
\label{sec:representation}

A process--bigraph may appear in three equivalent textual forms (Fig.~\ref{fig:pb-representations}):

\begin{enumerate}[noitemsep,topsep=2pt,leftmargin=1.5em]
    \item a JSON-like serialized document, which is the canonical stored format;
    \item a reduced tree notation, used in this supplement for readability;
    \item a linearized one-line syntax using bracketed annotations.
\end{enumerate}

These formats differ only in presentation.  
JSON and the linearized syntax can be parsed by the \texttt{Core} engine into the same in-memory executable composite, and round-trip conversion between them is deterministic and lossless.
The reduced tree notation is a human-readable rendering of the same structure, used here for clarity.

\begin{figure}[H]
\centering
\begin{tabular}{cc}

% ------------------------------------------------------------
% LEFT PANEL: JSON REPRESENTATION
% ------------------------------------------------------------
\begin{minipage}[t]{0.48\textwidth}
\vspace{0pt}
\scriptsize\ttfamily
\{\\
\hspace*{3mm}"schema": \{\\
\hspace*{7mm}"stores": \{\\
\hspace*{11mm}"store": "float"\\
\hspace*{7mm}\},\\
\hspace*{7mm}"processes": \{\\
\hspace*{11mm}"proc": \{\\
\hspace*{15mm}"inputs": ["store"],\\
\hspace*{15mm}"outputs": ["store"]\\
\hspace*{11mm}\}\\
\hspace*{7mm}\}\\
\hspace*{3mm}\},\\
\hspace*{3mm}"state": \{\\
\hspace*{7mm}"stores": \{\\
\hspace*{11mm}"store": 0.0\\
\hspace*{7mm}\}\\
\hspace*{3mm}\}\\
\}
\end{minipage}
&
% ------------------------------------------------------------
% RIGHT PANEL: REDUCED TREE REPRESENTATION
% ------------------------------------------------------------
\begin{minipage}[t]{0.48\textwidth}
\vspace{0pt}
\scriptsize\ttfamily
schema:\\
\hspace*{3mm}stores:\\
\hspace*{6mm}store: float\\
\hspace*{3mm}processes:\\
\hspace*{6mm}proc:\\
\hspace*{9mm}inputs: [store]\\
\hspace*{9mm}outputs: [store]\\[4pt]
state:\\
\hspace*{3mm}stores:\\
\hspace*{6mm}store: 0.0
\end{minipage}

\end{tabular}

\caption{\textbf{Equivalent representations of a simple process--bigraph.}
\emph{Left:} JSON-like serialized document.
\emph{Right:} Reduced tree notation used throughout this supplement.
The same structure can also be written in linearized form as:
\texttt{schema[stores[store:float]|processes[proc:inputs[store]|outputs[store]]]|\allowbreak state[stores[store:0.0]]}.}
\label{fig:pb-representations}
\end{figure}

% ------------------------------------------------------------
% 2.2 Types, Schema Trees, and State Trees
% ------------------------------------------------------------

\subsection{Types, schema trees, and state trees}
\label{sec:pb-schema-state}

A \emph{schema tree} is a partial map
\[
    \Sigma : \mathcal{P} \rightharpoonup \mathcal{T},
\]
assigning a type to each path in a JSON-like hierarchical structure.
Each $\Sigma(p)$ specifies the type governing the subtree rooted at~$p$.
Composite types appear at internal nodes and constrain the structure of their children.
Leaf types specify primitive values such as numbers, strings, or booleans.
A schema tree therefore determines field types, array shapes, port signatures, and the types of all \texttt{process} classes.

A \emph{state tree} is a partial map
\[
    x : \mathcal{P} \rightharpoonup \mathcal{V},
\]
assigning concrete values to paths.
Leaves at designated store paths correspond to the \emph{stores} of the system.
Internal nodes may be objects or arrays that organize the hierarchy.

A state tree $x$ is \emph{well-formed} for a schema tree $\Sigma$ when, for every path $p$ where both are defined, the value $x(p)$ is valid for the type declared at~$\Sigma(p)$.
We write this as the typing judgment
\[
    \Sigma \vdash x : \mathsf{State},
\]
which is read as: under the schema $\Sigma$, the state tree $x$ is a well-formed state.

Figure~\ref{fig:simple_schema_state} illustrates a simple schema tree (left) and a matching state tree (right), showing how the schema constrains the structure and types of the corresponding concrete values.

\begin{figure}[H]
\centering
\begin{tabular}{cc}

% ------------------------------------------------------------
% LEFT PANEL: SCHEMA TREE (REDUCED FORMAT)
% ------------------------------------------------------------
\begin{minipage}[t]{0.45\textwidth}
\vspace{0pt}
\scriptsize\ttfamily
organism:\\
\hspace*{3mm}cell:\\
\hspace*{6mm}volume: float (um\textsuperscript{3})\\
\hspace*{6mm}mass: float (pg)\\
\hspace*{3mm}environment:\\
\hspace*{6mm}temperature: float (K)\\
\hspace*{6mm}ph: float
\end{minipage}
&
% ------------------------------------------------------------
% RIGHT PANEL: STATE TREE (REDUCED FORMAT)
% ------------------------------------------------------------
\begin{minipage}[t]{0.45\textwidth}
\vspace{0pt}
\scriptsize\ttfamily
organism:\\
\hspace*{3mm}cell:\\
\hspace*{6mm}volume: 1.2\\
\hspace*{6mm}mass: 0.85\\
\hspace*{3mm}environment:\\
\hspace*{6mm}temperature: 310.0\\
\hspace*{6mm}ph: 7.2
\end{minipage}

\end{tabular}

\caption{\textbf{Example of schema and state trees in reduced textual format.}
\emph{Left:} schema hierarchy with unit-annotated leaf types.
\emph{Right:} matching state supplying concrete values consistent with the schema.
}
\label{fig:simple_schema_state}
\end{figure}

% ------------------------------------------------------------
% 2.3 Type Engine and Type Registry
% ------------------------------------------------------------

\subsubsection{Type engine and type registry}
The type engine (e.g.\ \texttt{bigraph-schema}~\texttt{Core}) maintains a global \texttt{type\_registry}, written $R_T$.
This registry defines all available types and their semantics, including:
\begin{itemize}[noitemsep,topsep=2pt,leftmargin=1.5em]
    \item validation and parsing of values,
    \item an update operator $\mathsf{apply}_\tau$ for each type $\tau \in \mathcal{T}$,
    \item serialization and deserialization methods.
\end{itemize}

Given a schema tree $\Sigma$ and state tree $x$, the type engine checks that the typing judgment $\Sigma \vdash x : \mathsf{State}$ holds.

% ------------------------------------------------------------
% 2.4 Links, Ports and Wiring
% ------------------------------------------------------------

\subsection{Links, ports and wiring}
\label{sec:pb-ports-wiring}

In \texttt{bigraph-schema}, a \emph{link} is a node whose schema specifies a set of typed input and output ports.  
Figure~\ref{fig:process_schema_state} shows a typical example: the schema for \texttt{"mm\_process"} declares two input ports (\texttt{"substrate"}, \texttt{"enzyme"}) and one output port (\texttt{"product"}), each annotated with a type.

Formally, for a link at path $p \in \mathcal{P}$, the schema tree $\Sigma$ determines:
\begin{itemize}[noitemsep,topsep=2pt,leftmargin=1.5em]
    \item its interface, with input ports $P_{\mathrm{in}}(p)$ and output ports $P_{\mathrm{out}}(p)$,
    \item for each port $\ell$, the declared type $\tau_\ell = \Sigma(p.\ell)$.
\end{itemize}

The corresponding state-tree representation is shown in Fig.~\ref{fig:process_schema_state} (right).  
A link node in the state tree $x$ stores:
\begin{itemize}[noitemsep,topsep=2pt,leftmargin=1.5em]
    \item \texttt{inputs}: mapping input-port names to the state paths where their values are read,
    \item \texttt{outputs}: mapping output-port names to the state paths where their updates are written,
    \item \texttt{config}: process-specific parameters.
\end{itemize}
For example, the \texttt{mm\_process} \texttt{"substrate"} input port is wired to \texttt{["state","substrate\_conc"]}, and \texttt{"product"} is wired to \texttt{["state","product\_conc"]}.

From these \texttt{inputs} and \texttt{outputs} fields the global wiring pattern is obtained.  The wiring map is therefore not stored separately: it is \emph{derived} from the collection of link nodes in~$x$.

Formally, collecting these entries across all link paths yields:
\[
    W : (\mathsf{LinkPath} \times \mathsf{PortName}) \to \mathcal{P},
\]
where $W(p,\ell)$ returns the state-tree path connected to port~$\ell$ of the link at $p$, and $\mathsf{LinkPath}$ is the set of paths whose schema entries denote links or their specializations (e.g.\ \texttt{process}, \texttt{step}, \texttt{composite}).

Wiring is \emph{well-typed} when each port is connected to a state path whose schema type matches the port’s declared type.  
For instance, the \texttt{"substrate"} input of the Michaelis--Menten process must be wired to a store typed as \texttt{float (mM)} in~$\Sigma$.

\begin{figure}[H]
\centering
\begin{tabular}{cc}

% ------------------------------------------------------------
% LEFT PANEL: PROCESS SCHEMA TREE (REDUCED FORMAT)
% ------------------------------------------------------------
\begin{minipage}[t]{0.45\textwidth}
\vspace{0pt}
\scriptsize\ttfamily
mm\_process:\\
\hspace*{3mm}\_type: process\\
\hspace*{3mm}\_inputs:\\
\hspace*{6mm}substrate: float (mM)\\
\hspace*{6mm}enzyme: float (mM)\\
\hspace*{3mm}\_outputs:\\
\hspace*{6mm}product: float (mM)\\
\hspace*{3mm}config:\\
\hspace*{6mm}kcat: float (1/s)\\
\hspace*{6mm}Km: float (mM)\\
\hspace*{3mm}address: protocol\\
\hspace*{3mm}interval: float (s)
\end{minipage}
&
% ------------------------------------------------------------
% RIGHT PANEL: PROCESS STATE TREE (REDUCED FORMAT)
% ------------------------------------------------------------
\begin{minipage}[t]{0.45\textwidth}
\vspace{0pt}
\scriptsize\ttfamily
mm\_process:\\
\hspace*{3mm}inputs:\\
\hspace*{6mm}substrate: [state, substrate\_conc]\\
\hspace*{6mm}enzyme: [state, enzyme\_conc]\\
\hspace*{3mm}outputs:\\
\hspace*{6mm}product: [state, product\_conc]\\
\hspace*{3mm}config:\\
\hspace*{6mm}kcat: 1.2\\
\hspace*{6mm}Km: 0.5\\
\hspace*{3mm}address: local:MichaelisMenten\\
\hspace*{3mm}interval: 0.1
\end{minipage}

\end{tabular}

\caption{\textbf{Example of a process schema and matching state in reduced textual format.}
\emph{Left:} schema for a Michaelis--Menten process, including typed ports, configuration fields, and metadata.
\emph{Right:} corresponding state that binds ports to store paths, assigns numeric parameters, and selects a concrete implementation via the \texttt{address} field.
}
\label{fig:process_schema_state}
\end{figure}

% ------------------------------------------------------------
% 2.5 Processes and Delta Semantics
% ------------------------------------------------------------

\subsection{Processes and delta semantics}
\label{sec:pb-processes-deltas}

\subsubsection{Process nodes and the link registry}

\texttt{process-bigraph} extends the generic typed-link structure by introducing \texttt{Process}, \texttt{Step}, and \texttt{Composite} as \emph{specialized} link types.  
Like all links, a process node inherits typed input and output ports and participates in the global wiring map~$W$; it additionally carries the fields needed for runtime execution.  

These fields are:
\begin{itemize}[noitemsep,topsep=2pt,leftmargin=1.5em]
    \item an \texttt{address} identifying a handler class in the \texttt{link\_registry},
    \item a typed \texttt{config} subtree describing its parameters,
    \item an \texttt{interval} declaring its nominal time advance,
    \item typed input/output port declarations inherited from the schema.
\end{itemize}

The \emph{link registry} $R_L : \mathsf{Address} \to \mathsf{HandlerClass}$ maps each address to a concrete handler class.  
Initialization instantiates the handler using the node’s \texttt{config} and stores the instance at the same path $p_{\mathrm{proc}}$ in the in-memory state tree.  
Thus the schema determines what kind of process may appear, while the handler instance determines how that process behaves at runtime.  

\paragraph{Process interfaces as typed function signatures.}

At the schema level, every process node specifies a \emph{typed interface} describing what it consumes and what it produces.  
This can be written as a function signature
\[
\mathsf{process}_{p_{\mathrm{proc}}}\bigl(\text{config}^{\tau_c}\bigr) :
\bigl(\text{in}_{1}^{\tau_{i1}}, \text{in}_{2}^{\tau_{i2}}, \dots\bigr)
\;\longrightarrow\;
\bigl(\text{out}_{1}^{\tau_{o1}}, \text{out}_{2}^{\tau_{o2}}, \dots\bigr).
\]
This signature expresses the process contract: its configuration space $\tau_c$, the types of values it may read, and the types of values it may update.  

\paragraph{Processes as delta generators.}

At runtime, the instantiated handler implements this signature via an \texttt{update} method.  
Abstractly, this has the form
\[
\mathsf{update} :
\bigl(\text{config}^{\tau_c}, \text{in}_{1}^{\tau_{i1}}, \dots\bigr)
\;\longrightarrow\;
\Delta,
\]
returning a \emph{composite delta} $\Delta$, a tree-structured object whose shape mirrors the process’s output schema and whose leaves are typed deltas associated with individual output ports.  
In this way, the schema-level view (typed function signature) and the runtime view (delta-producing handler) align: both describe the same transformation, one abstractly and one operationally.

\subsubsection{Deltas and type-directed application}

For each type $\tau \in \mathcal{T}$, the type engine defines a type-specific update operator
\[
    \mathsf{apply}_\tau : \mathcal{V}_\tau \times \Delta_\tau \to \mathcal{V}_\tau,
\]
where $\Delta_\tau$ is the class of deltas valid for~$\tau$.  
Deltas describe \emph{how} a value should change.  
Each type determines the shape of its permissible deltas, how to apply them, and what counts as a well-formed update.  

We distinguish three broad categories of deltas.  

\paragraph{1. Primitive deltas.}

Primitive deltas are the \emph{leaf-level} updates applied to values of non-structured types.  
For such leaf types, a primitive delta typically encodes a direct change --- such as an increment, logical update, or replacement.  
Applying a primitive delta updates the associated store value directly:
\[
x' = \mathsf{apply}_\tau(x, \delta).
\]

\paragraph{2. Composite deltas.}

Structured types (records, arrays, maps) carry \emph{tree-structured} deltas that mirror the shape of the composite value.  
A composite delta may contain primitive deltas at leaves, nested composite deltas at interior nodes, and optionally structural edit instructions.  
A process’s \texttt{update} method usually returns such a delta tree, whose top-level branches correspond to its output ports.  
After wiring distributes these deltas to the appropriate state paths, each leaf is applied using the appropriate $\mathsf{apply}_\tau$ operator.  

\paragraph{3. Structural deltas.}

Structural deltas modify the \emph{shape} of either the state tree or the schema tree.  
They include:
\begin{itemize}[noitemsep,topsep=2pt,leftmargin=1.5em]
    \item \textbf{insert}: add a new subtree,
    \item \textbf{delete}: remove a subtree,
    \item \textbf{move}: relocate a subtree,
    \item \textbf{rewrite}: modify fields, types, shapes, or metadata,
    \item \textbf{rewire}: modify \texttt{inputs}/\texttt{outputs} so ports point to different stores.
\end{itemize}
Since processes, ports, schedule entries, and wiring tables all appear as subtrees, these edits naturally express graph rewrites such as division, merging, engulfment, or spawning.  
They require no special orchestration rules: they are applied through the same type-directed delta semantics as numerical updates.

\subsubsection{Single-process update protocol}

A single update step for a process located at path $p_{\mathrm{proc}}$ unfolds as follows.  

\paragraph{1. Input projection.}

For each input port~$\ell$, the wiring map~$W$ specifies the source state path.  
The runtime gathers the current input values:
\[
    x_{\mathrm{in}}(\ell)
    = x\bigl(W(p_{\mathrm{proc}}, \ell)\bigr).
\]

\paragraph{2. Evaluation.}

Given the timestep $\Delta t$ chosen by the orchestration policy (Section~\ref{sec:pb-orchestration}), the handler instance computes
\[
    \delta
    = \mathsf{update}_{p_{\mathrm{proc}}}(x_{\mathrm{in}}, \Delta t),
\]
yielding a composite delta whose fields mirror the process’s output ports.  

\paragraph{3. Application.}

For each output port~$\ell$, let $q = W(p_{\mathrm{proc}},\ell)$ be the target state path and let $\tau = \Sigma(q)$ be its declared type.  
The type engine then applies the delta using the type-directed rule
\[
        x'(q)
        = \mathsf{apply}_\tau\bigl(x(q),\, \delta(\ell)\bigr).
\]
Applying all such deltas yields a new state tree $x'$ that remains well-typed with respect to the schema~$\Sigma$.  

\medskip

In summary, processes behave as typed function signatures at the schema level, handler instances with update methods at runtime, and generators of typed deltas that the type engine applies uniformly across numerical, structural, and graph-rewrite updates.  
This unification is what enables process bigraphs to support heterogeneous modeling methods and dynamic structural change within a single execution semantics.

% ------------------------------------------------------------
% 2.5 Process Bigraph Definition
% ------------------------------------------------------------

\subsection{Explicit definition of a Process--Bigraph}

We can now summarize the core ingredients of the framework as a single structure.

A \emph{Process--Bigraph} is a tuple
\[
    B = (\Sigma, x, R_T, R_L),
\]
consisting of:
\begin{enumerate}[noitemsep,topsep=0pt,leftmargin=1.5em]
    \item $\Sigma : \mathcal{P} \rightharpoonup \mathcal{T}$, a schema tree assigning a type to each path in a JSON-like hierarchy;
    \item $x : \mathcal{P} \rightharpoonup \mathcal{V}$, a state tree assigning concrete values to paths, including the \texttt{inputs}, \texttt{outputs}, and handler instances stored at link and process nodes;
    \item $R_T$, the type registry providing validation and type-directed update operators $\mathsf{apply}_\tau$ for each type $\tau$;
    \item $R_L$, the link registry mapping process addresses to handler classes, from which configured process instances are created and stored in $x$.
\end{enumerate}

A global wiring map $W$ is \emph{derived} from the \texttt{inputs} and \texttt{outputs} fields stored in the state tree~$x$ for each link node.

These components must satisfy the following consistency conditions:
\begin{itemize}[noitemsep,topsep=2pt,leftmargin=1.5em]
    \item \textbf{Type correctness:}  
          The typing judgment $\Sigma \vdash x : \mathsf{State}$ holds: whenever both $\Sigma(p)$ and $x(p)$ are defined, $x(p)$ is valid for the type declared at $\Sigma(p)$.
    \item \textbf{Well-typed wiring:}  
          For every link node and port~$\ell$, the schema type declared for that port matches the schema type at its destination path obtained from the derived wiring map~$W$.
    \item \textbf{Well-formed processes:}  
          Each process node in $\mathsf{LinkPath}$ has a valid \texttt{address} pointing to a handler class in $R_L$, and the state tree contains a corresponding configured handler instance stored at the same path.
\end{itemize}

A Process--Bigraph is therefore a fully typed, wired, and executable structure, ready to be advanced in time by the orchestration semantics described in Section~\ref{sec:pb-orchestration}.

% ------------------------------------------------------------
% 2.6 Composites
% ------------------------------------------------------------

\subsection{Composites}
\label{sec:pb-composites}

A \texttt{Composite} is a specialized \texttt{process} that serves as the main simulation engine for \texttt{process-bigraph}.  
Its configuration encodes an entire process--bigraph --- a schema tree, a state tree, and the registries needed to interpret them --- so that a composite
behaves as a full, self-contained simulation when executed.  
An example is shown in Fig.~\ref{fig:composite_process}.

A composite is also a process, that connect its internal process--bigraph to an external state.
It does this with two addition attributes:
\begin{itemize}[noitemsep,topsep=2pt,leftmargin=1.5em]
    \item declares an \texttt{interface}, consisting of typed input and output ports just like any other process node;
    \item declares a \texttt{bridge} mapping these external ports to internal state-tree paths within the embedded bigraph.
\end{itemize}
The interface specifies the composite’s external API, while the \texttt{bridge} acts as the inward-facing wiring.  
The type of each interface port must match the schema type at its internal bridge destination.

At runtime, the composite’s configuration stores:
\begin{itemize}[noitemsep,topsep=2pt,leftmargin=2em]
    \item the embedded schema tree $\Sigma_{\mathrm{state}}$,
    \item the embedded state tree $x_{\mathrm{state}}$, including all internal link and process nodes,
    \item the global \texttt{type\_registry} $R_T$,
    \item the global \texttt{link\_registry} $R_L$, providing handler classes for processes.
\end{itemize}
As in the top-level case, the internal wiring pattern is not stored separately: it is \emph{derived} from the \texttt{inputs} and \texttt{outputs} fields of link nodes within $x_{\mathrm{state}}$.

Operationally, a composite $C$ is identified as
\[
    C = \bigl(
        \Sigma_{\mathrm{state}},\;
        x_{\mathrm{state}},\;
        R_T,\;
        R_L,\;
        \mathsf{bridge},\;
        \mathsf{interface}
    \bigr),
\]
with internal wiring implicitly determined by~$x_{\mathrm{state}}$.

Under orchestration (Section~\ref{sec:pb-orchestration}), a composite behaves as a standard process externally: values arriving at its interface ports are routed inward through the \texttt{bridge}, internal processes advance according to their scheduling rules, and outgoing deltas are returned through the external ports.  
Composites thus provide hierarchical modularity: externally a single process, internally a complete process--bigraph.

\begin{figure}[H]
\centering
\begin{tabular}{cc}

% ------------------------------------------------------------
% LEFT PANEL: STATE TREE
% ------------------------------------------------------------
\begin{minipage}[t]{0.3\textwidth}
\vspace{0pt}
\scriptsize\ttfamily
process1:\\
\hspace*{3mm}outputs:\\
\hspace*{6mm}port1: [store1.1]\\
\hspace*{6mm}port2: [store1.2]\\[4pt]

process2:\\
\hspace*{3mm}outputs:\\
\hspace*{6mm}port1: [store1.1]\\
\hspace*{6mm}port2: [store1.2]\\[4pt]

bridge:\\
\hspace*{3mm}inputs:\\
\hspace*{6mm}port1: [store1.1]\\
\hspace*{6mm}port2: [store1.2]
\end{minipage}
&
% ------------------------------------------------------------
% RIGHT PANEL: DIAGRAM
% ------------------------------------------------------------
\begin{minipage}[t]{0.3\textwidth}
\vspace{0pt}
\centering
\includegraphics[
    height=5.5cm,
    keepaspectratio,
    trim=0 0 0 75,
    clip
]{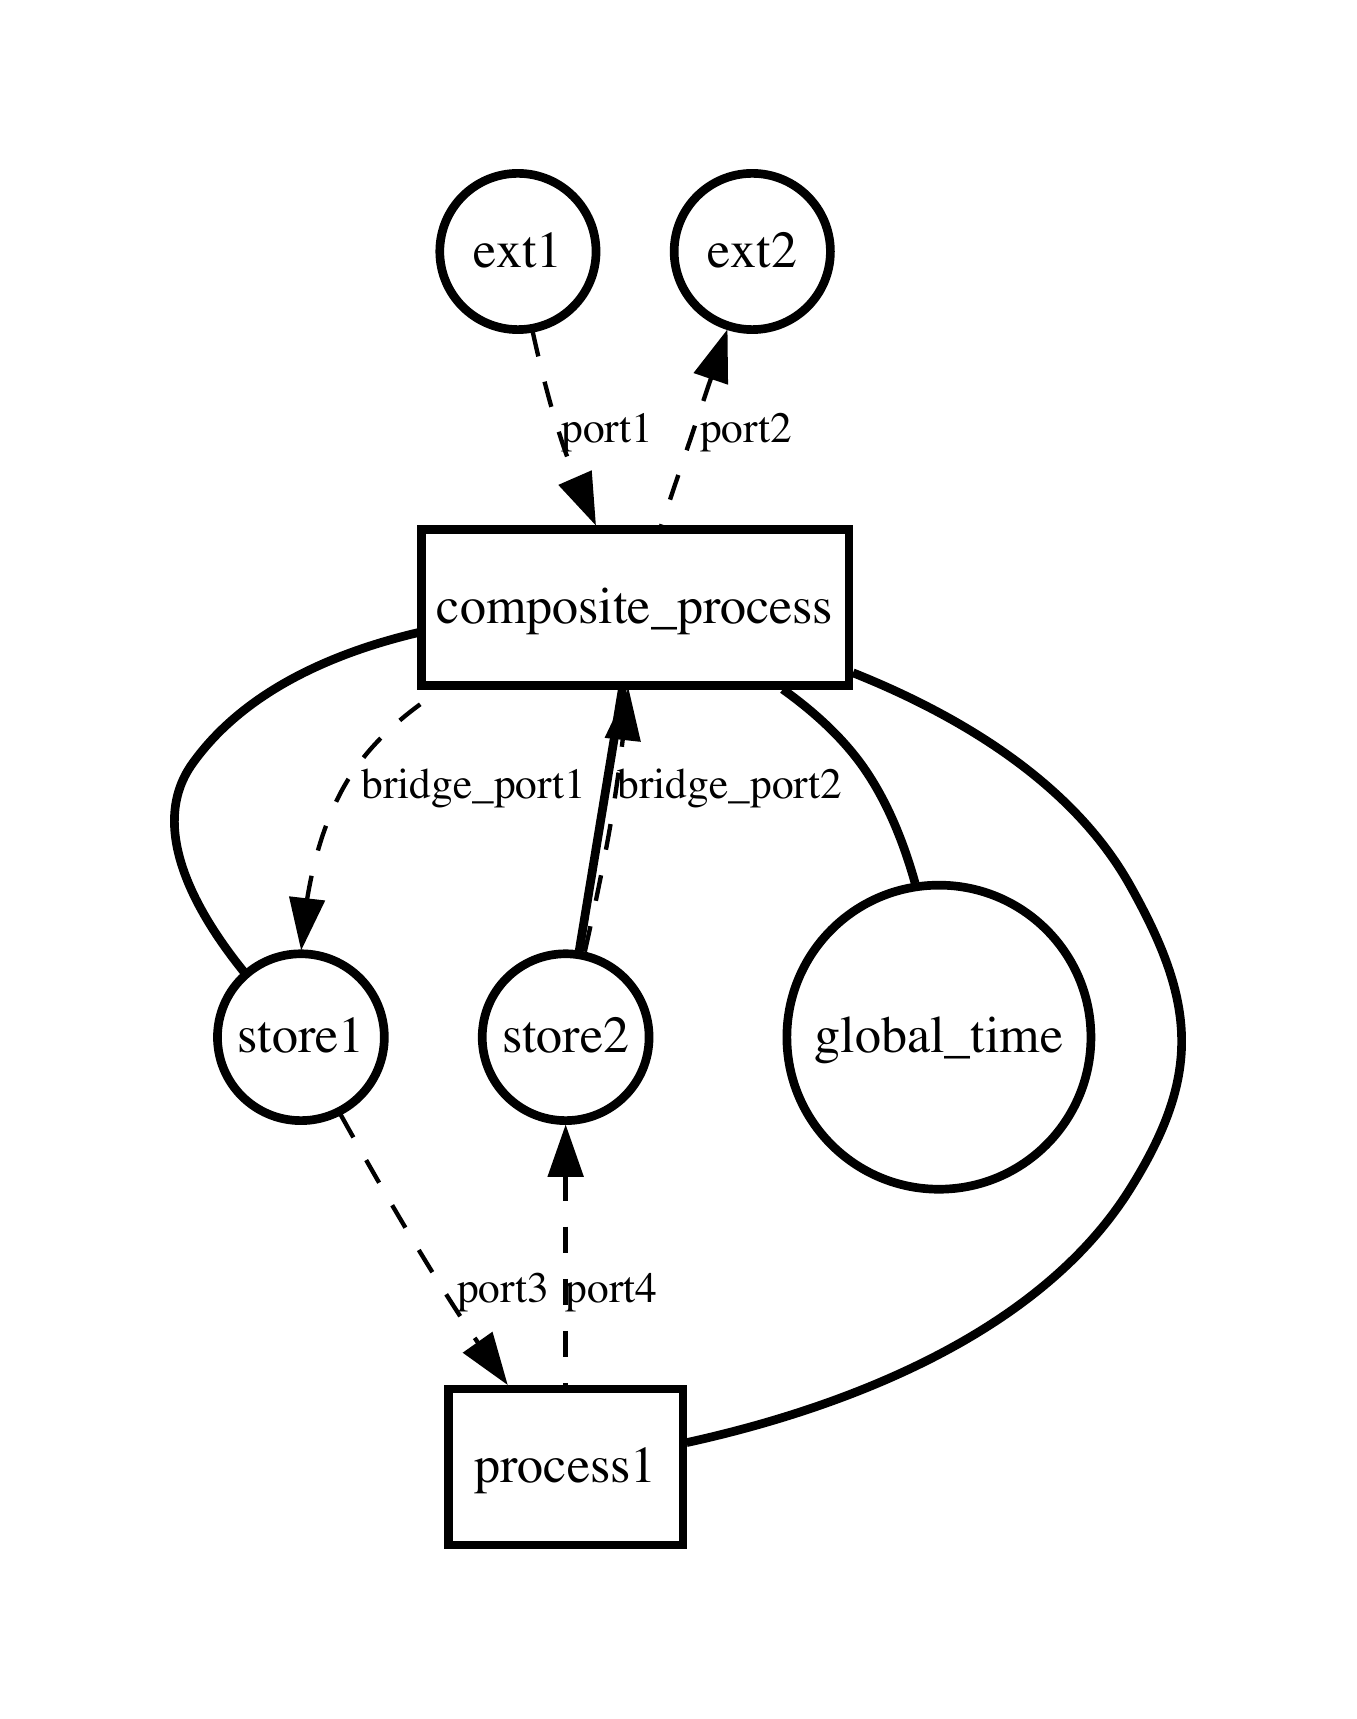}
\end{minipage}

\end{tabular}
\caption{\textbf{State tree and diagram of a composite process.}
\emph{Left:} a state tree instantiating the declared ports and connecting them to stores.
\emph{Right:} the resulting process bigraph visualized with \texttt{bigraph-viz}.
}
\label{fig:composite_process}
\end{figure}

% ------------------------------------------------------------
% 2.7 Orchestration (Event scheduling, workflows, rewrites)
% ------------------------------------------------------------
\subsection{Orchestration}
\label{sec:pb-orchestration}

The orchestration pattern used by the \texttt{Composite} class follows the spirit of the Discrete Event System Specification (DEVS), in which simulation components can declare their own time advance, and a global orchestrator repeatedly executes the next imminent event.  
In our setting, these ideas are reinterpreted for typed process--bigraphs:  components become process nodes with typed ports, and transitions become type-directed updates over schema/state trees.

\subsubsection{Event times and schedule}

Each process node $p \in \mathsf{LinkPath}$ carries:
\begin{itemize}[noitemsep,topsep=2pt,leftmargin=1.5em]
    \item an \emph{interval} value $\mathsf{interval}(p)$ declaring its nominal time advance;
    \item an \emph{address} linking it to a handler class in the \texttt{link\_registry} $R_L$ (whose configured instance is stored at $p$ in the state tree);
    \item typed input and output ports whose wiring is determined by the \texttt{inputs}/\texttt{outputs} entries in the state tree.
\end{itemize}

At runtime, the composite maintains:
\begin{itemize}[noitemsep,topsep=2pt,leftmargin=1.5em]
    \item a global time $t \in \mathbb{R}_{\ge 0}$,
    \item a schedule $t_{\mathrm{next}} : \mathsf{LinkPath} \to \mathbb{R}_{\ge 0}$
          assigning each process node its next event time.
\end{itemize}
Initially, one may set $t_{\mathrm{next}}(p) = t_0 + \mathsf{interval}(p)$ for
an initial time $t_0$.

\subsubsection{Small-step orchestration semantics}

A configuration is a triple
\[
    \langle B, t, t_{\mathrm{next}} \rangle,
\]
where $B = (\Sigma, x, R_T, R_L)$ is a well-typed Process--Bigraph, $t$ is the current time, and $t_{\mathrm{next}}$ is the current schedule.

We define a transition
\[
    \langle B, t, t_{\mathrm{next}} \rangle
    \;\longrightarrow\;
    \langle B', t', t_{\mathrm{next}}' \rangle
\]
by the following rules.

\paragraph{(Select) Scheduler step.}
Let
\[
  t^\star = \min_{p \in \mathsf{LinkPath}}\, t_{\mathrm{next}}(p)
\]
be the next event time.
Let
\[
  S = \{\, p \in \mathsf{LinkPath} \mid t_{\mathrm{next}}(p) = t^\star \,\}
\]
be the set of all processes whose events occur at $t^\star$.
We advance the global time to $t' = t^\star$.
All processes in $S$ then undergo a \emph{Process Update}, conceptually in parallel when their deltas commute.

\paragraph{(Process Update).}
For each $p \in S$ --- all processes updating at the same event time $t^\star$ --- the runtime performs:
\begin{enumerate}[noitemsep,topsep=0pt,leftmargin=1.5em]
  \item Perform input projection by reading the state paths listed in the \texttt{inputs} field at $p$, yielding $x_{\mathrm{in}}$.
  \item Invoke the configured handler instance stored at path $p$:
        \[
            \delta_p = \mathsf{update}_p(x_{\mathrm{in}},\, \Delta t),
        \]
        where $\Delta t = t^\star - t$.
        The result $\delta_p$ is a (possibly composite) delta structured by the output ports of $p$.
  \item Apply $\delta_p$ to the state paths listed in the \texttt{outputs} field of $p$ using the type engine’s $\mathsf{apply}_\tau$ operators.
\end{enumerate}
Collectively applying all deltas $\{\delta_p \mid p \in S\}$ yields the updated state tree $x'$ and schema tree $\Sigma'$.
This produces the updated Process--Bigraph $B' = (\Sigma', x', R_T, R_L)$, with internal wiring re-derived from the updated \texttt{inputs}/\texttt{outputs} fields.

\paragraph{(Reschedule).}
For each process node $p$ that persists in $B'$, set
\[
  t_{\mathrm{next}}'(p) = t' + \mathsf{interval}(p),
\]
unless overridden by process-specific semantics (e.g.\ disabling or pausing a process).
Process nodes created or removed by structural deltas update the domain of $t_{\mathrm{next}}'$ accordingly.

\subsubsection{DAG-structured discrete workflows}
\label{sec:pb-dag-workflows}

If all processes in a subsystem satisfy $\mathsf{interval}(p)=0$, scheduling reduces to a directed acyclic graph (DAG) evaluation over these \texttt{step} nodes, with edges determined by data dependencies in the wiring.

Within a single global time $t$, execution proceeds as follows:
\begin{itemize}[noitemsep,topsep=2pt,leftmargin=1.5em]
    \item a step $p$ becomes \emph{eligible} when all input ports updated in this tick have received new values;
    \item inputs unchanged in this tick do not block execution, allowing partially updated data to propagate;
    \item execution proceeds in topological order: once a step applies its output deltas, any successor steps whose inputs changed become eligible.
\end{itemize}
Cycles are disallowed, ensuring deterministic zero-time DAG evaluation within the broader event-scheduling semantics.

Because \texttt{Composite} nodes can behave like ordinary processes, an entire composite simulation can itself appear as a single \texttt{step} in a larger DAG.
This enables end-to-end workflows in which multiple simulations and other tools such as parameter estimation and analysis can be integrated within the same framework.

\subsubsection{Recursive composition}

Because a \texttt{Composite} encapsulates its own scheduler, stores, and internal processes, it acts externally as a process but internally executes a complete process--bigraph.
For temporal processes inside the composite, the internal scheduler maintains its own event queue, advancing the front of that schedule in time and updating the embedded state and schema as structural deltas create, remove, or move process nodes.
The composite therefore continually re-tracks all available internal processes, their paths, and their next update times.
After each internal update, the composite advances its own event time according to its interval field, and outward-facing results are propagated through its interface ports via the \texttt{bridge}.
In this way, temporal dynamics, DAG-style workflows, and structural graph rewrites coexist naturally within a single hierarchical system under uniform schema-based, typed-link semantics.

\subsection{Emitters and result capture}

Emitters are special \texttt{step} processes whose role is observational of the simulation state for saving results.
An emitter declares typed input ports, but no semantic outputs back into the simulation state.
At execution time, the emitter reads values from its input ports and records them into an external or side-channel store for later retrieval, analysis, or visualization.

Operationally, an emitter participates in orchestration exactly like any other step process:
when scheduled, it performs input projection, invokes its handler, and produces a delta.
However, the delta produced by an emitter is it writing to a recording backend (e.g.\ in-memory buffers, disk, streaming logs), rather than as an update to the schema/state tree.
Emitters therefore do not introduce new data dependencies into the process--bigraph and cannot affect subsequent process execution.

\clearpage

% ============================================================
% S3 Spatio–Flux instantiation of the semantics
% ============================================================

\section{Spatio--Flux Instantiation}
\label{sec:pb-spatioflux-instantiation}

This section gives a concrete, example of the Process--Bigraph  semantics introduced in Section~\ref{sec:process-bigraphs} applied to the Spatio--Flux example from the main text.
We begin by introducing some of Spatio--Flux's types in \ref{sec:spatioflux-types} and processes in \ref{sec:spatioflux-processes}.
These are then integrated for the reference demonstration in \ref{sec:spatioflux-composite}, with all the required config parameters and wiring.
All documents and tests for this example are available in the public \texttt{spatio-flux} repository, as well as many other novel compositions.

% ============================================================
% SPATIO-FLUX TYPES
% ============================================================

\subsection{Spatio--Flux types}
\label{sec:spatioflux-types}

Spatio--Flux instantiates the abstract schema/state semantics of Section~\ref{sec:pb-schema-state} using two classes of domain-specific stores: \texttt{fields} and \texttt{particles}.  
These stores serve as the primary state objects of the Spatio--Flux model.  
% Table~\ref{tab:spatioflux-stores} summarizes these stores at a glance.  
% Figure~\ref{fig:spatioflux_types} illustrates how the complex particle and fields types occupy the schema/state trees.  
Throughout this section, we use the term \emph{store} for a top-level state-tree entry (\texttt{fields} or \texttt{particles}) and \emph{type} for the schema that describes the values stored there, which includes \texttt{concentrations}, \texttt{volume}, \texttt{mass}, and \texttt{position}, amongst others.  
The types are displayed on individual cards for easier viewing.

% ------------------------------------------------------------
% FIELD-RELATED TYPES
% ------------------------------------------------------------

\subsubsection{Field-related types}

\begin{sfxtypecard}{conc_counts}{Concentration--counts record}{fields}
All molecular species in the environment are represented using a typed \texttt{conc\_counts} record.
This record stores the molecular amount as counts, the containing volume, and the derived concentration.

\begin{sfxtypefields}{conc\_counts}
  \sfxfieldrow{volume}{float}
  \sfxfieldrow{counts}{float}
  \sfxfieldrow{concentration}{float}
\end{sfxtypefields}

\noindent\textbf{Semantics and usage.}
\begin{itemize}[nosep]
  \item Counts and concentration are inter-convertible: if one is updated, the other is automatically adjusted to remain consistent.
  \item Volume deltas rescale the existing amount before concentration is recomputed.
  \item Non-negativity is enforced by clamping negative total amounts to zero.
\end{itemize}
\end{sfxtypecard}

\begin{sfxtypecard}{fields}{Fields store}{fields}
The \texttt{fields} store maps each substrate identifier to a two-dimensional array of \texttt{conc\_counts} sites.
This structure represents the spatial distribution of each environmental chemical species.

\begin{sfxtypefields}{fields}
  \sfxfieldrow{value}{array with shape \([n_x, n_y]\), entries of type \texttt{conc\_counts}}
\end{sfxtypefields}

\noindent\textbf{Semantics and usage.}
\begin{itemize}[nosep]
  \item Each substrate (e.g.\ \texttt{"glucose"} or \texttt{"acetate"}) is associated with one typed lattice of \texttt{conc\_counts} sites.
  \item Field-based processes such as diffusion and Monod kinetics operate by reading and writing typed deltas on these arrays.
\end{itemize}
\end{sfxtypecard}

% ------------------------------------------------------------
% PARTICLE-RELATED TYPES
% ------------------------------------------------------------

\subsubsection{Particle-related types}

\begin{sfxtypecard}{particle}{Base particle}{particles}
The \texttt{particle} type provides the minimal particle interface, including identification, spatial position, mass, and metabolic subfields for sensing and exchange.
This type captures the core positional state and local metabolic environment shared by all particle agents in Spatio--Flux.

\begin{sfxtypefields}{particle}
  \sfxfieldrow{id}{string}
  \sfxfieldrow{position}{position}
  \sfxfieldrow{mass}{concentration}
  \sfxfieldrow{local}{map of concentration}
  \sfxfieldrow{exchange}{map of counts}
\end{sfxtypefields}

\noindent\textbf{Semantics and usage.}
\begin{itemize}[nosep]
  \item The \texttt{local} field stores concentrations sensed from nearby field sites and is updated by the \texttt{particle\_exchange} bridge process.
  \item The \texttt{exchange} field stores flux-like count deltas that will be injected into the corresponding lattice cell during particle--field exchange.
  \item Position provide the basic state for mechanical processes, and mass can updated by metabolic processes.
\end{itemize}
\end{sfxtypecard}

\begin{sfxtypecard}{complex_particle}{Complex particle extension}{particles}
The \texttt{complex\_particle} type extends the base particle interface with mechanical attributes such as shape, velocity, inertia, friction, elasticity, and radius.
This type supports Newtonian dynamics when used with the Pymunk-based movement process.

\begin{sfxtypefields}{complex\_particle}
  \sfxfieldrow{\_inherit}{particle}
  \sfxfieldrow{shape}{enum\{circle, segment\}}
  \sfxfieldrow{velocity}{tuple of floats (x, y)}
  \sfxfieldrow{inertia}{float}
  \sfxfieldrow{friction}{float}
  \sfxfieldrow{elasticity}{float}
  \sfxfieldrow{radius}{float}
\end{sfxtypefields}

\noindent\textbf{Semantics and usage.}
\begin{itemize}[nosep]
  \item The \texttt{\_inherit} field indicates that all fields of \texttt{particle} are available in addition to the mechanical attributes.
  \item Shape, radius, and inertia determine how particles interact with walls and barriers in the Newtonian integrator.
  \item Velocity, friction, and elasticity control continuous movement, damping, and collisions within the physics engine.
\end{itemize}
\end{sfxtypecard}

\begin{sfxtypecard}{particles}{Particle agents}{particles}
The \texttt{particles} store is a typed map from each particle identifier to a \texttt{complex\_particle} record.
Particle processes read and write these records directly and may perform structural rewrites such as division or boundary removal.

\begin{sfxtypefields}{particles}
  \sfxfieldrow{value}{map[particle]}
\end{sfxtypefields}

\noindent\textbf{Semantics and usage.}
\begin{itemize}[nosep]
  \item Each entry (e.g.\ \texttt{"p\_9afa18"}) corresponds to a single particle or cell aggregate.
  \item Brownian and Newtonian movement processes update positions and mechanical fields of these records through typed deltas.
  \item Graph-rewrite processes such as \texttt{particle\_division} add and remove entries in this map to model birth, death, and division events.
\end{itemize}
\end{sfxtypecard}

% ============================================================
% SPATIO-FLUX PROCESSES
% ============================================================

\subsection{Spatio--Flux processes}
\label{sec:spatioflux-processes}

Spatio--Flux instantiates the Process Bigraph semantics through a small set of processes that can be wired into the \texttt{fields} and/or \texttt{particles} stores.  
Each process is a \texttt{process} or \texttt{step} node whose schema specifies typed input and output ports and whose state-tree entry stores its \texttt{address}, \texttt{config}, and wiring to concrete store paths.  
Upon execution, each process receives an input projection, computes an update delta tree, and applies it using the type engine’s \(\mathsf{apply}\) operators, as formalized in Section~\ref{sec:pb-processes-deltas}.

\begin{table}[H]
  \centering
  \renewcommand{\arraystretch}{1.25}
  \begin{tabular}{p{0.2\textwidth} p{0.26\textwidth} p{0.46\textwidth}}
    \hline
    \textbf{Process family} & \textbf{Processes} & \textbf{Role in composite simulations} \\
    \hline

    Metabolic processes &
    \texttt{DynamicFBA}, \texttt{MonodKinetics}, \texttt{SpatialDFBA} &
    Compute metabolic uptake, secretion, and biomass production at single sites or across spatially distributed locations by operating on substrate fields and biomass variables. \\

    Field transport &
    \texttt{DiffusionAdvection} &
    Updates dissolved species fields through diffusion and advection, coupling metabolic activity across space. \\

    Particle movement &
    \texttt{BrownianMovement}, \texttt{PymunkParticleMovement} &
    Updates particle positions in continuous space. Brownian motion provides stochastic movement, while Newtonian motion introduces mass, velocity, inertia, friction, and elastic interactions. \\

    Particle--field coupling &
    \texttt{ParticleExchange} &
    Mediates bidirectional exchange between particle-local state and spatial fields, synchronizing internal particle chemistry with nearby lattice values. \\

    Structural and boundary processes &
    \texttt{ParticleDivision}, \texttt{ManageBoundaries} &
    Rewrites the particle store by creating, removing, or relocating particles in response to state-dependent conditions such as growth thresholds or boundary crossings. \\

    \hline
  \end{tabular}
  \caption{
    \textbf{Spatio--Flux process families.}
    Each family encapsulates a distinct modeling concern—metabolism, transport, motion, exchange, or structural change—that can be composed through typed interfaces.
    More complex simulations arise by combining families rather than extending any single process.
  }
  \label{tab:spatioflux-processes}
\end{table}

% ------------------------------------------------------------
% 1. METABOLIC PROCESSES
% ------------------------------------------------------------

\subsubsection{Local metabolic processes}

Metabolic processes operate on individual lattice sites, which store derived concentrations.
Each metabolic process reads local substrate concentrations and biomass, computes reaction rates, and writes back typed count deltas to the same site, ensuring compatibility with the \texttt{conc\_counts} update semantics.
Because the metabolic processes share a common typed interface, they can be interchanged freely at any lattice location.

% ------------------------------------------------------------
% Monod kinetics card
% ------------------------------------------------------------
\begin{sfxprocesscard}{monod\_kinetics}{Monod kinetics (ODE)}{process}{local metabolic}
The \texttt{monod\_kinetics} process provides a saturating-rate ODE for uptake and secretion at a single lattice site.
It implements the \texttt{metabolism} interface with a compact configuration in terms of reactions and kinetic parameters.

\begin{sfxprocessinterface}{monod\_kinetics}{process}
  \sfxprocport{biomass}{input}{concentration}
  \sfxprocport{substrates}{input}{map[concentration]}
  \sfxprocport{biomass}{output}{counts}
  \sfxprocport{substrates}{output}{map[counts]}
\end{sfxprocessinterface}

\begin{sfxprocessparams}
  \sfxprocparam{reactions}{map[reaction]}{\texttt{\{assimilate\_glucose, maintenance\_turnover\}}}{Reaction definitions mapping \texttt{reactant} and \texttt{product} species for each Monod term.}
  \sfxprocparam{kinetic\_params}{map[tuple[float,float]]}{\(\texttt{glucose}:(0.5,0.01);\; \texttt{mass}:(1.0,0.001)\)}{Per-species Monod parameters \((K_m, V_{\max})\) for substrate uptake and mass turnover.}
\end{sfxprocessparams}

\noindent\textbf{Semantics and equations.}
For each configured Monod term with reactant \(R\) (a substrate concentration \(c_R\), or biomass \(m\) if \(R=\texttt{mass}\)) and product \(P\), the site-local rate is
\[
  v_R \;=\; \frac{V_{\max,R}\, c_R}{K_{m,R} + c_R}.
\]
Over timestep \(\Delta t\), the process returns stoichiometric deltas in \texttt{counts} form:
reactant is consumed \(\Delta N_R = -v_R\Delta t\), biomass increases when \(P=\texttt{mass}\) via \(\Delta m = v_R\Delta t\), and any product substrate \(S\) receives \(\Delta N_S = +v_R\Delta t\).

\end{sfxprocesscard}

% ------------------------------------------------------------
% dFBA card
% ------------------------------------------------------------
\begin{sfxprocesscard}{dfba}{Dynamic FBA (network-level metabolism)}{process}{local metabolic}
The \texttt{dfba} process uses a full metabolic network model and computes feasible instantaneous fluxes using \texttt{cobraPy}.
It implements the same \texttt{metabolism} interface as \texttt{monod\_kinetics}, but with a configuration that points to a COBRA model and specifies how substrates are mapped to exchange reactions.

\begin{sfxprocessinterface}{dfba}{process}
  \sfxprocport{biomass}{input}{concentration}
  \sfxprocport{substrates}{input}{map[concentration]}
  \sfxprocport{biomass}{output}{counts}
  \sfxprocport{substrates}{output}{map[counts]}
\end{sfxprocessinterface}

\begin{sfxprocessparams}
  \sfxprocparam{model\_file}{string}{required}{Path to the COBRA metabolic model used for FBA.}
  \sfxprocparam{kinetic\_params}{map[tuple[float,float]]}{required}{Per-substrate Michaelis--Menten parameters \((K_m, V_{\max})\) used to set uptake bounds.}
  \sfxprocparam{substrate\_update\_reactions}{map[string]}{required}{Map from substrate identifiers to exchange reaction IDs in the model.}
  \sfxprocparam{bounds}{map[bounds]}{required}{Optional overrides for exchange-reaction lower/upper bounds.}
\end{sfxprocessparams}

\noindent\textbf{Semantics and equations.}
For each substrate \(s\) with concentration \(c_s\), an uptake bound is computed via Michaelis--Menten kinetics and applied to the corresponding exchange reaction:
\[
  v_{s}^{\mathrm{uptake}} \;=\; -\frac{V_{\max,s}\, c_s}{K_{m,s} + c_s}.
\]
Given bounds \(\ell \le v \le u\), the COBRA model solves an instantaneous FBA problem (typically maximizing growth), yielding an optimal growth rate \(\mu\) and exchange fluxes \(v_s\).
The returned \texttt{counts}-typed deltas over \(\Delta t\) are
\[
  \Delta m \;=\; \mu\, m\, \Delta t,
  \qquad
  \Delta N_s \;=\; v_s\, m\, \Delta t,
\]
with substrate deltas clamped to preserve non-negativity under \texttt{conc\_counts} semantics.

\end{sfxprocesscard}

% ------------------------------------------------------------
% 2. FIELD PROCESSES
% ------------------------------------------------------------
\subsubsection{Field movement}

Field movement processes operate on the two-dimensional arrays of typed \texttt{conc\_counts} sites stored in the \texttt{fields} map.
Each species occupies a lattice of concentrations, and the field processes update these concentrations by computing spatial fluxes and returning typed deltas that the \texttt{conc\_counts} \texttt{\_apply} operator converts into consistent \texttt{counts} and \texttt{concentration} updates.
Because the interface is typed, field processes integrate seamlessly into the Process--Bigraph semantics: inputs project each species array, the handler computes spatial fluxes, and outputs return per-site deltas under the \texttt{fields} port.

\begin{sfxprocesscard}{diffusion}{Diffusion--advection}{process}{field movement}
The \texttt{diffusion} process updates the concentration fields of all substrates on the spatial lattice using an explicit advection--diffusion scheme.
It reads the current concentration arrays for each species and returns typed deltas that modify the same arrays in place.

\begin{sfxprocessinterface}{diffusion}{process}
  \sfxprocport{fields}{input}{map[array[concentration]]}
  \sfxprocport{fields}{output}{map[array[concentration]]}
\end{sfxprocessinterface}

\begin{sfxprocessparams}
  \sfxprocparam{n\_bins}{tuple[integer,integer]}{required}{Number of lattice cells in \((x,y)\).}
  \sfxprocparam{bounds}{tuple[float,float]}{required}{Physical domain size in \((L_x, L_y)\).}
  \sfxprocparam{default\_diffusion\_rate}{float}{\texttt{1e-1}}{Default diffusion coefficient \(D\) used if no species-specific value is given.}
  \sfxprocparam{diffusion\_coeffs}{map[float]}{none}{Per-species diffusion coefficients overriding the default.}
  \sfxprocparam{advection\_coeffs}{map[tuple[float,float]]}{none}{Per-species advection velocities \((v_x, v_y)\).}
  \sfxprocparam{max\_dt}{float}{\texttt{1e-1}}{Upper bound on internal diffusion timestep.}
  \sfxprocparam{cfl\_adv}{float}{\texttt{0.5}}{CFL stability factor for the advection term.}
  \sfxprocparam{clip\_negative}{boolean}{\texttt{true}}{If true, negative concentrations are clipped to zero.}
\end{sfxprocessparams}

\noindent\textbf{Semantics and equations.}
For each species field \(C_s\), concentrations evolve according to
\[
  \partial_t C_s \;=\; D_s \nabla^2 C_s \;-\; \mathbf{v}_s \cdot \nabla C_s.
\]
The handler selects a stable internal timestep \(\delta t\) (CFL-limited and capped by \texttt{max\_dt}) and advances the field with \(n=\lceil \Delta t/\delta t\rceil\) explicit Euler substeps using standard finite-difference stencils.
The emitted output is a per-species delta array
\[
  \Delta C_s = C_s^{\mathrm{final}} - C_s^{\mathrm{initial}},
\]
optionally clipped to enforce non-negative concentrations.

\end{sfxprocesscard}

% ------------------------------------------------------------
% 3. PARTICLE MOVEMENT PROCESSES
% ------------------------------------------------------------
\subsubsection{Particle movement processes}

Particle movement processes operate on the \texttt{particles} store, a typed map from particle identifiers to particle records.
The schema distinguishes base \texttt{particle} records from \texttt{complex\_particle} records that also include mechanical attributes (shape, velocity, inertia, friction, elasticity, radius).
Each movement process is a typed \texttt{process} node whose ports are wired to \texttt{particles} and whose update method returns deltas that modify particle attributes and, when needed, perform structural rewrites on the particle map.

\begin{sfxprocesscard}{brownian\_movement}{Brownian movement}{process}{particle movement}
The \texttt{brownian\_movement} process models overdamped drift--diffusion of
particles inside a rectangular domain.
It acts on base \texttt{particle} records and updates only the
\texttt{position} field of each surviving particle, with optional boundary
birth/death.

\begin{sfxprocessinterface}{brownian\_movement}{process}
  \sfxprocport{particles}{input}{map[particle]}
  \sfxprocport{particles}{output}{map[particle]}
\end{sfxprocessinterface}

\begin{sfxprocessparams}
  \sfxprocparam{bounds}{tuple[float,float]}{required}{Spatial domain size used to clamp particle positions.}
  \sfxprocparam{diffusion\_rate}{float}{\texttt{1e-1}}{Brownian diffusion coefficient \(D\).}
  \sfxprocparam{advection\_rate}{tuple[float,float]}{(0.0, 0.0)}{Uniform drift velocity \((v_x, v_y)\).}
\end{sfxprocessparams}

\noindent\textbf{Semantics and equations.}
Each particle position \(X_i \in \mathbb{R}^2\) is updated over \(\Delta t\) using an Euler--Maruyama drift--diffusion step:
\[
  X_i \leftarrow X_i + \mathbf{v}\,\Delta t + \sqrt{2D\,\Delta t}\,\xi_i,
  \qquad \xi_i \sim \mathcal{N}(0,I_2).
\]
The process emits typed deltas that update only the \texttt{position} field of each particle.
Particles that cross configured absorbing boundaries may be removed via structural \texttt{\_remove} deltas when boundary-driven rewrites are enabled; otherwise, positions are unconstrained by the process itself.

\end{sfxprocesscard}

\begin{sfxprocesscard}{newtonian\_particles}{Newtonian particles}{process}{particle movement}
The \texttt{newtonian\_particles} process refines particle mechanics by treating each particle as a rigid body in a 2D physics engine (Pymunk).
It acts on \texttt{complex\_particle} records with explicit mechanical attributes and updates both positions and velocities, with optional boundary birth/death.

\begin{sfxprocessinterface}{newtonian\_particles}{process}
  \sfxprocport{particles}{input}{map[particle]}
  \sfxprocport{particles}{output}{map[particle]}
\end{sfxprocessinterface}

\begin{sfxprocessparams}
  \sfxprocparam{bounds}{tuple[float,float]}{(500.0, 500.0)}{Physical domain size for particle motion.}
  \sfxprocparam{diffusion\_rate}{float}{\texttt{1e-1}}{Effective mechanical diffusion strength (jitter scale).}
  \sfxprocparam{advection\_rate}{tuple[float,float]}{(0.0, 0.0)}{Global drift velocity applied to all particles.}
  \sfxprocparam{substeps}{integer}{\texttt{100}}{Number of Pymunk substeps per external timestep.}
  \sfxprocparam{damping\_per\_second}{float}{\texttt{0.98}}{Global velocity damping per second.}
  \sfxprocparam{gravity}{float}{\texttt{-9.81}}{Vertical gravitational acceleration.}
  \sfxprocparam{friction}{float}{\texttt{0.8}}{Contact friction coefficient.}
  \sfxprocparam{elasticity}{float}{\texttt{0.0}}{Contact elasticity (bounciness).}
  \sfxprocparam{jitter\_per\_second}{float}{\texttt{1e-2}}{Standard deviation of random impulse per second.}
  \sfxprocparam{barriers}{list[map]}{\texttt{[]}}{Optional internal obstacles/walls definitions.}
  \sfxprocparam{wall\_thickness}{float}{\texttt{100.0}}{Thickness of outer domain walls.}
\end{sfxprocessparams}

\noindent\textbf{Semantics and equations.}
Particles are simulated as rigid bodies governed by Newtonian mechanics,
\[
  m\,\frac{dV}{dt} = F_{\mathrm{net}},
  \qquad
  \frac{dX}{dt} = V,
\]
implemented via a 2D physics engine with configured gravity, damping, contact mechanics, and stochastic jitter.
Over an external timestep \(\Delta t\), the engine advances in multiple substeps, after which the process emits deltas updating particle positions, velocities, and other mechanical attributes.
Boundary crossings may additionally trigger \texttt{\_add}/\texttt{\_remove} rewrites on the particle map.
\end{sfxprocesscard}

% ------------------------------------------------------------
% Boundary management card
% ------------------------------------------------------------
\begin{sfxprocesscard}{manage\_boundaries}{Manage boundaries (reflect \& absorb)}{step}{boundary policy}
The \texttt{manage\_boundaries} step enforces boundary policies on particle \emph{absolute} positions.
It reads the \texttt{particles} map, applies absorbing removal for configured sides, reflects all other out-of-range coordinates back into the domain interior, and can spawn new particles at selected boundaries according to a Poisson birth process.

\begin{sfxprocessinterface}{manage\_boundaries}{step}
  \sfxprocport{particles}{input}{map[particle]}
  \sfxprocport{process\_interval}{input}{float}
  \sfxprocport{particles}{output}{map[particle]}
\end{sfxprocessinterface}

\begin{sfxprocessparams}
  \sfxprocparam{bounds}{tuple[float,float]}{required}{Domain size \((L_x,L_y)\) defining hard bounds \([0,L_x]\times[0,L_y]\).}
  \sfxprocparam{add\_rate}{float}{\texttt{0.0}}{Birth event rate (1/sec) used to sample boundary-spawn events.}
  \sfxprocparam{boundary\_to\_add}{list[boundary\_side]}{\texttt{["top"]}}{Sides where new particles may be spawned.}
  \sfxprocparam{boundary\_to\_remove}{list[boundary\_side]}{\texttt{[]}}{Absorbing sides; particles crossing a configured side are removed.}
  \sfxprocparam{buffer}{float}{\texttt{1e-6}}{Numerical buffer used to reflect into the interior to avoid floating-point sticking on walls.}
  \sfxprocparam{mass\_range}{tuple[float,float]}{\texttt{INITIAL\_MASS\_RANGE}}{Mass range used when generating newborn particles.}
\end{sfxprocessparams}

\noindent\textbf{Semantics and equations.}
Let the hard domain be \([0,L_x]\times[0,L_y]\) and the interior reflection domain be
\([\,\epsilon,\,L_x-\epsilon\,]\times[\,\epsilon,\,L_y-\epsilon\,]\) with \(\epsilon=\texttt{buffer}\).
For each particle id \(i\) with absolute position \(X_i=(x_i,y_i)\):

\begin{enumerate}[noitemsep,topsep=0pt,leftmargin=1.5em]
\item \emph{Absorbing removal.} If \(X_i\) violates a configured absorbing side
(e.g.\ \(x_i<0\) when \texttt{left} is absorbing, \(x_i>L_x\) when \texttt{right} is absorbing, etc.),
emit a structural \texttt{\_remove} delta for \(i\).

\item \emph{Reflection.} Otherwise, any out-of-range coordinate is reflected back into the interior interval.
In one dimension, reflection into \([lo,hi]\) is computed by
\[
  \mathrm{reflect}(x;lo,hi)
  \;=\;
  \begin{cases}
    lo + y, & y \le (hi-lo)\\
    hi - (y-(hi-lo)), & y > (hi-lo)
  \end{cases}
  \qquad
  y = (x-lo)\bmod 2(hi-lo),
\]
and applied componentwise:
\[
  (x_i',y_i') =
  \bigl(\mathrm{reflect}(x_i;\epsilon,L_x-\epsilon),\;
        \mathrm{reflect}(y_i;\epsilon,L_y-\epsilon)\bigr).
\]
Emit an \emph{absolute} position update delta for particle \(i\):
\(\Delta_i = \{\texttt{position}:(x_i',y_i')\}\).
\end{enumerate}

\emph{Boundary births.}
Let \(\Delta t=\texttt{process\_interval}\) and birth rate \(\lambda=\texttt{add\_rate}\).
For each boundary \(b \in \texttt{boundary\_to\_add}\), sample an event with probability
\[
  p_{\mathrm{birth}} = 1 - e^{-\lambda \Delta t}.
\]
On success, generate a new id \(j\), choose an absolute spawn position \(X_j\) on side \(b\),
sample mass from \texttt{mass\_range}, and emit a structural \texttt{\_add} delta inserting the new particle record.

The output under \texttt{particles} therefore combines (i) attribute deltas for absolute position updates,
and (ii) structural edits \texttt{\_remove}/\texttt{\_add} implementing absorbing boundaries and Poisson births.
\end{sfxprocesscard}

% \noindent\textbf{Boundary-driven graph rewrites.}
% Both Brownian and Newtonian movement can optionally perform graph rewrites at the domain boundaries by adding or removing particle entries in the \texttt{particles} map.
% Boundary removal is handled by marking particles that cross configured absorbing sides of the domain for deletion, producing a \texttt{\_remove} branch in the particle delta tree.
% Boundary-driven births are triggered by probabilistic rules that insert new particle records near selected sides as \texttt{\_add} deltas.
% These operations demonstrate how continuous mechanical dynamics and discrete topological changes coexist in the same Process--Bigraph: positions and velocities are updated via typed field deltas, whereas entry and exit at boundaries are expressed as structural edits to the underlying particle graph.

% \begin{sfxprocessparams}
%   \sfxprocparam{add\_probability}{float}{\texttt{0.0}}{Probability of spawning a new particle at selected boundaries.}
%   \sfxprocparam{boundary\_to\_add}{list[boundary\_side]}{\texttt{["top"]}}{Sides of the domain where new particles can appear.}
%   \sfxprocparam{boundary\_to\_remove}{list[boundary\_side]}{["left","right", "top","bottom"]}{Absorbing boundaries where particles are removed.}
% \end{sfxprocessparams}

% ------------------------------------------------------------
% 4. PARTICLE–FIELD EXCHANGE
% ------------------------------------------------------------
\subsubsection{Particle--field exchange as an adapter}

\begin{sfxprocesscard}{particle\_exchange}{Particle--field exchange}{step}{adapter}
\texttt{particle\_exchange} is a \texttt{step} node that acts as an adapter between the particle representation and the field lattice.
It has ports on both \texttt{particles} and \texttt{fields} but introduces no new physics of its own; instead, it synchronizes state between the two stores in a typed way.

\begin{sfxprocessinterface}{particle\_exchange}{step}
  \sfxprocport{particles}{input}{map[particle]}
  \sfxprocport{fields}{input}{fields}
  \sfxprocport{particles}{output}{map[particle]}
  \sfxprocport{fields}{output}{fields}
\end{sfxprocessinterface}

\begin{sfxprocessparams}
  \sfxprocparam{bounds}{tuple[float,float]}{required}{Domain bounds used to map particle positions to lattice indices.}
  \sfxprocparam{n\_bins}{tuple[integer,integer]}{required}{Number of lattice cells in \((x,y)\); must match the \texttt{fields} grid.}
\end{sfxprocessparams}

\noindent\textbf{Semantics and equations.}
Each particle position \(x_i\) is mapped to a lattice cell \((c_i,r_i)\).
Let \(C_m(c,r)\) denote the field concentration of species \(m\) at that cell.
The adapter synchronizes particle-local and field representations by (i) updating each particle’s stored local snapshot from \(C_m(c_i,r_i)\), and (ii) applying queued per-particle exchange amounts \(f_{i,m}\) as field deltas
\[
  \Delta C_m(c_i,r_i) \;{+}{=}\; f_{i,m}.
\]
Consumed exchange entries are reset to zero via particle deltas, ensuring one-shot transfer semantics.

\end{sfxprocesscard}

% ------------------------------------------------------------
% 5. PARTICLE DIVISION
% ------------------------------------------------------------
\subsubsection{Particle division as a graph rewrite}

\begin{sfxprocesscard}{particle\_division}{Particle division}{step}{graph rewrite}
The \texttt{particle\_division} process is a \texttt{step} node whose primary role is to demonstrate graph rewrites on the \texttt{particles} store.
It has a purely particle-based interface and performs no continuous time integration; instead, it rewrites the particle map whenever a mass threshold is exceeded.

\begin{sfxprocessinterface}{particle\_division}{step}
  \sfxprocport{particles}{input}{map[particle]}
  \sfxprocport{particles}{output}{map[particle]}
\end{sfxprocessinterface}

\begin{sfxprocessparams}
  \sfxprocparam{division\_mass\_threshold}{float}{\texttt{0.0}}{Mass threshold above which particles are eligible to divide (disabled if \(\le 0\)).}
  \sfxprocparam{division\_jitter}{float}{\texttt{1e-3}}{Fraction of a reference length used as jitter radius to place daughter particles.}
\end{sfxprocessparams}
\noindent\textbf{Semantics and equations.}
For each particle with mass \(m_i \ge m_{\mathrm{thr}}\), the process performs a graph rewrite:
the parent particle is removed and two daughters are inserted.
Daughter positions are displaced symmetrically by a small random offset, and masses split the parent mass,
\[
  m_{i,1} = m_{i,2} = \tfrac{1}{2} m_i.
\]
All changes are emitted as \texttt{\_remove} and \texttt{\_add} deltas on the \texttt{particles} map.
\end{sfxprocesscard}

% ============================================================
% SPATIO-FLUX COMPOSITES
% ============================================================
\subsection{Particle--COMETS composition}
\label{sec:spatioflux-composite}

The Spatio--Flux reference demonstration is instantiated as a single \texttt{Composite} (\texttt{particle\_comets}).
Its schema declares top-level stores for \texttt{fields}, \texttt{particles}, and \texttt{global\_time}, together with a collection of process and step nodes whose ports are wired into these stores.

At the environment level, \texttt{diffusion} (\texttt{DiffusionAdvection}) advances dissolved species fields on a $10\times 10$ lattice with configurable diffusion/advection coefficients and boundary conditions.
A grid of \texttt{monod\_kinetics[i,j]} processes (\texttt{MonodKinetics}) operates locally at each lattice site, consuming and producing substrates and updating \texttt{dissolved biomass} as a field variable.
Particle motion is handled by \texttt{newtonian\_particles} (\texttt{PymunkParticleMovement}), which updates positions and mechanical attributes (e.g., shape, radius, velocity, friction, elasticity) for each entry of the \texttt{particles} map.

The coupling between particles and fields is mediated by \texttt{particle\_exchange} (\texttt{ParticleExchange}), which maps continuous particle positions to lattice indices and synchronizes per-particle \texttt{local} concentrations and \texttt{exchange} counts with the spatial \texttt{fields}.
Two structural steps enforce population-level dynamics: \texttt{enforce\_boundaries} (\texttt{ManageBoundaries}) adds/removes particles at domain boundaries at a rate tied to the particle-motion interval, and \texttt{particle\_division} (\texttt{ParticleDivision}) rewrites the particle map when particles exceed a mass threshold.

Within each particle, metabolic growth is itself compositional: two internal dFBA processes (\texttt{DynamicFBA})—both modified \textit{E.~coli} core models with complementary substrate preferences—update particle-local exchange fluxes and organism-specific submasses.
An \texttt{aggregate\_mass} adapter accumulates these submasses into the particle’s total \texttt{mass}, providing the scalar growth signal monitored by \texttt{particle\_division}.

% =======================
% diffusion
% =======================
\begin{sfxcompositecard}{particle\_comets}
  \begin{sfxcompositeprocess}{diffusion}{process diffusion}{field transport}

    \begin{sfxcompositewires}
      \sfxwire{fields}{input}{fields}
      \sfxwire{fields}{output}{fields}
    \end{sfxcompositewires}

    \begin{sfxcompositeprops}
      \sfxprop{address}{local.DiffusionAdvection}
      \sfxprop{interval}{1.0}
    \end{sfxcompositeprops}

    \begin{sfxconfigtable}
      \sfxconfigrow{bounds}{[50.0, 50.0]}
      \sfxconfigrow{n\_bins}{[10, 10]}
      \sfxconfigrow{default\_diffusion\_rate}{0.1}
      \sfxconfigrow{default\_diffusion\_dt}{0.1}
      \sfxconfigrow{max\_dt}{0.1}
      \sfxconfigrow{cfl\_adv}{0.5}
      \sfxconfigrow{clip\_negative}{true}

      \sfxconfigrow{diffusion\_coeffs.glucose}{0.1}
      \sfxconfigrow{diffusion\_coeffs.acetate}{0.1}
      \sfxconfigrow{diffusion\_coeffs.dissolved\ biomass}{0.1}

      \sfxconfigrow{advection\_coeffs.glucose}{[0.0, 0.0]}
      \sfxconfigrow{advection\_coeffs.acetate}{[0.0, 0.0]}
      \sfxconfigrow{advection\_coeffs.dissolved\ biomass}{[0.0, 0.0]}

      \sfxconfigrow{boundary\_conditions.default.x.type}{periodic}
      \sfxconfigrow{boundary\_conditions.default.y.type}{neumann}
      \sfxconfigrow{boundary\_conditions.glucose.top.type}{dirichlet}
      \sfxconfigrow{boundary\_conditions.glucose.top.value}{5.0}
      \sfxconfigrow{boundary\_conditions.acetate.bottom.type}{dirichlet}
      \sfxconfigrow{boundary\_conditions.acetate.bottom.value}{5.0}
    \end{sfxconfigtable}

  \end{sfxcompositeprocess}
\end{sfxcompositecard}

% =======================
% monod_kinetics[i,j]
% =======================
\begin{sfxcompositecard}{particle\_comets}
  \begin{sfxcompositeprocess}{monod\_kinetics[i,j]}{process monod\_kinetics}{local metabolic}

    \begin{sfxcompositewires}
      \sfxwire{substrates.glucose}{input}{fields.glucose[i,j]}
      \sfxwire{substrates.acetate}{input}{fields.acetate[i,j]}
      \sfxwire{biomass}{input}{fields.dissolved\ biomass[i,j]}

      \sfxwire{substrates.glucose}{output}{fields.glucose[i,j]}
      \sfxwire{substrates.acetate}{output}{fields.acetate[i,j]}
      \sfxwire{biomass}{output}{fields.dissolved\ biomass[i,j]}
    \end{sfxcompositewires}

    \begin{sfxcompositeprops}
      \sfxprop{address}{local.MonodKinetics}
      \sfxprop{interval}{1.0}
    \end{sfxcompositeprops}

    \begin{sfxconfigtable}
      \sfxconfigrow{reactions.assimilate\_glucose.reactant}{glucose}
      \sfxconfigrow{reactions.assimilate\_glucose.product}{mass}
      \sfxconfigrow{reactions.assimilate\_glucose.km}{1.0}
      \sfxconfigrow{reactions.assimilate\_glucose.vmax}{0.02}
      \sfxconfigrow{reactions.assimilate\_glucose.yield}{0.15}

      \sfxconfigrow{reactions.overflow\_to\_acetate.reactant}{glucose}
      \sfxconfigrow{reactions.overflow\_to\_acetate.product}{acetate}
      \sfxconfigrow{reactions.overflow\_to\_acetate.km}{1.0}
      \sfxconfigrow{reactions.overflow\_to\_acetate.vmax}{0.2}
      \sfxconfigrow{reactions.overflow\_to\_acetate.yield}{0.85}

      \sfxconfigrow{reactions.maintenance\_turnover.reactant}{mass}
      \sfxconfigrow{reactions.maintenance\_turnover.product}{detritus}
      \sfxconfigrow{reactions.maintenance\_turnover.km}{1.0}
      \sfxconfigrow{reactions.maintenance\_turnover.vmax}{0.001}
      \sfxconfigrow{reactions.maintenance\_turnover.yield}{1.0}
    \end{sfxconfigtable}

  \end{sfxcompositeprocess}
\end{sfxcompositecard}

% =======================
% newtonian_particles
% =======================
\begin{sfxcompositecard}{particle\_comets}
  \begin{sfxcompositeprocess}{newtonian\_particles}{process newtonian\_particles}{particle movement}

    \begin{sfxcompositewires}
      \sfxwire{particles}{input}{particles}
      \sfxwire{particles}{output}{particles}
    \end{sfxcompositewires}

    \begin{sfxcompositeprops}
      \sfxprop{address}{local.PymunkParticleMovement}
      \sfxprop{interval}{1.0}
    \end{sfxcompositeprops}

    \begin{sfxconfigtable}
      \sfxconfigrow{bounds}{[50.0, 50.0]}
      \sfxconfigrow{substeps}{100}
      \sfxconfigrow{gravity}{-1.0}
      \sfxconfigrow{damping\_per\_second}{0.95}
      \sfxconfigrow{jitter\_per\_second}{0.01}
      \sfxconfigrow{diffusion\_rate}{0.1}
      \sfxconfigrow{advection\_rate}{[0.0, 0.0]}

      \sfxconfigrow{friction}{0.9}
      \sfxconfigrow{elasticity}{0.1}
      \sfxconfigrow{wall\_thickness}{100.0}
      \sfxconfigrow{barriers}{[]}

      \sfxconfigrow{new\_particle\_radius\_range}{[0.5, 2.0]}
      \sfxconfigrow{new\_particle\_mass\_range}{[1.0, 1.0]}
      \sfxconfigrow{new\_particle\_density}{0.015}
      \sfxconfigrow{new\_particle\_speed\_range}{[0.0, 0.0]}

      \sfxconfigrow{circle\_density}{0.015}
      \sfxconfigrow{segment\_radius}{10.0}
      \sfxconfigrow{segment\_density}{0.02}
      \sfxconfigrow{segment\_radius}{10.0}
      \sfxconfigrow{n\_bins}{[1, 1]}
    \end{sfxconfigtable}

  \end{sfxcompositeprocess}
\end{sfxcompositecard}

% =======================
% particle_exchange
% =======================
\begin{sfxcompositecard}{particle\_comets}
  \begin{sfxcompositeprocess}{particle\_exchange}{step particle\_exchange}{particle--field coupling}

    \begin{sfxcompositewires}
      \sfxwire{particles}{input}{particles}
      \sfxwire{fields}{input}{fields}
      \sfxwire{particles}{output}{particles}
      \sfxwire{fields}{output}{fields}
    \end{sfxcompositewires}

    \begin{sfxcompositeprops}
      \sfxprop{address}{local.ParticleExchange}
      \sfxprop{interval}{1.0}
    \end{sfxcompositeprops}

    \begin{sfxconfigtable}
      \sfxconfigrow{bounds}{[50.0, 50.0]}
      \sfxconfigrow{n\_bins}{[10, 10]}
      \sfxconfigrow{apply\_mass\_balance}{false}
      \sfxconfigrow{rates\_are\_per\_time}{true}
    \end{sfxconfigtable}

  \end{sfxcompositeprocess}
\end{sfxcompositecard}

% =======================
% enforce_boundaries
% =======================
\begin{sfxcompositecard}{particle\_comets}
  \begin{sfxcompositeprocess}{enforce\_boundaries}{step enforce\_boundaries}{boundary management}

    \begin{sfxcompositewires}
      \sfxwire{particles}{input}{particles}
      \sfxwire{process\_interval}{input}{newtonian\_particles.interval}
      \sfxwire{particles}{output}{particles}
    \end{sfxcompositewires}

    \begin{sfxcompositeprops}
      \sfxprop{address}{local.ManageBoundaries}
      \sfxprop{interval}{1.0}
    \end{sfxcompositeprops}

    \begin{sfxconfigtable}
      \sfxconfigrow{bounds}{[50.0, 50.0]}
      \sfxconfigrow{buffer}{0.0001}
      \sfxconfigrow{clamp\_survivors}{true}
      \sfxconfigrow{mass\_range}{[0.001, 1.0]}
      \sfxconfigrow{add\_rate}{0.0}
      \sfxconfigrow{boundary\_to\_remove}{[]}
      \sfxconfigrow{boundary\_to\_add}{["top","top","bottom","left","right"]}
    \end{sfxconfigtable}

  \end{sfxcompositeprocess}
\end{sfxcompositecard}

% =======================
% particle_division
% =======================
\begin{sfxcompositecard}{particle\_comets}
  \begin{sfxcompositeprocess}{particle\_division}{step particle\_division}{graph rewrite}

    \begin{sfxcompositewires}
      \sfxwire{particles}{input}{particles}
      \sfxwire{particles}{output}{particles}
    \end{sfxcompositewires}

    \begin{sfxcompositeprops}
      \sfxprop{address}{local.ParticleDivision}
      \sfxprop{interval}{1.0}
    \end{sfxcompositeprops}

    \begin{sfxconfigtable}
      \sfxconfigrow{division\_mass\_threshold}{0.4}
      \sfxconfigrow{division\_jitter}{0.001}
      \sfxconfigrow{sub\_mass\_split}{equal}
      \sfxconfigrow{submass\_split\_mode}{random}
    \end{sfxconfigtable}

  \end{sfxcompositeprocess}
\end{sfxcompositecard}

% =======================
% ecoli_1 dFBA (inside each particle)
% =======================
\begin{sfxcompositecard}{particle\_internal}
  \begin{sfxcompositeprocess}{ecoli\_1\ dFBA}{process ecoli\_1 dFBA}{particle metabolic}

    \begin{sfxcompositewires}
      \sfxwire{substrates}{input}{local}
      \sfxwire{biomass}{input}{sub\_masses.ecoli\_1}
      \sfxwire{substrates}{output}{exchange}
      \sfxwire{biomass}{output}{sub\_masses.ecoli\_1}
    \end{sfxcompositewires}

    \begin{sfxcompositeprops}
      \sfxprop{address}{local.DynamicFBA}
    \end{sfxcompositeprops}

    \begin{sfxconfigtable}
      \sfxconfigrow{model\_file}{textbook}
      \sfxconfigrow{kinetic\_params.glucose}{[0.1, 2.0]}
      \sfxconfigrow{kinetic\_params.acetate}{[1.0, 0.1]}
      \sfxconfigrow{substrate\_update\_reactions.glucose}{EX\_glc\_\_D\_e}
      \sfxconfigrow{substrate\_update\_reactions.acetate}{EX\_ac\_e}
      \sfxconfigrow{bounds.ATPM.lower}{1.0}
      \sfxconfigrow{bounds.ATPM.upper}{1.0}
      \sfxconfigrow{bounds.EX\_o2\_e.lower}{-2.0}
    \end{sfxconfigtable}

  \end{sfxcompositeprocess}
\end{sfxcompositecard}

% =======================
% ecoli_2 dFBA (inside each particle)
% =======================
\begin{sfxcompositecard}{particle\_internal}
  \begin{sfxcompositeprocess}{ecoli\_2\ dFBA}{process ecoli\_2 dFBA}{particle metabolic}

    \begin{sfxcompositewires}
      \sfxwire{substrates}{input}{local}
      \sfxwire{biomass}{input}{sub\_masses.ecoli\_2}
      \sfxwire{substrates}{output}{exchange}
      \sfxwire{biomass}{output}{sub\_masses.ecoli\_2}
    \end{sfxcompositewires}

    \begin{sfxcompositeprops}
      \sfxprop{address}{local.DynamicFBA}
    \end{sfxcompositeprops}

    \begin{sfxconfigtable}
      \sfxconfigrow{model\_file}{textbook}
      \sfxconfigrow{kinetic\_params.glucose}{[1.0, 0.1]}
      \sfxconfigrow{kinetic\_params.acetate}{[0.01, 1.0]}
      \sfxconfigrow{substrate\_update\_reactions.glucose}{EX\_glc\_\_D\_e}
      \sfxconfigrow{substrate\_update\_reactions.acetate}{EX\_ac\_e}
      \sfxconfigrow{bounds.ATPM.lower}{1.0}
      \sfxconfigrow{bounds.ATPM.upper}{1.0}
      \sfxconfigrow{bounds.EX\_o2\_e.lower}{-2.0}
    \end{sfxconfigtable}

  \end{sfxcompositeprocess}
\end{sfxcompositecard}

% =======================
% aggregate_mass (inside each particle)
% =======================
\begin{sfxcompositecard}{particle\_internal}
  \begin{sfxcompositeprocess}{aggregate\_mass}{process aggregate\_mass}{mass adapter}

    \begin{sfxcompositewires}
      \sfxwire{sub\_masses}{input}{sub\_masses}
      \sfxwire{total\_mass}{output}{mass}
    \end{sfxcompositewires}

    \begin{sfxcompositeprops}
      \sfxprop{address}{local.ParticleTotalMass}
    \end{sfxcompositeprops}

    \begin{sfxconfigtable}
      % empty config in spec
    \end{sfxconfigtable}

  \end{sfxcompositeprocess}
\end{sfxcompositecard}

\vspace{4mm}
\printbibliography

\end{document}
